# Supplementary material for: Stable Matching: Choosing Which Proposals to Make
Source: arXiv:2204.04162 source file (2023-05-01)
Supplement: Supplementary file 1 [file appendix-table-of-contents.tex]

\section*{Table of Contents, Appendix}

\bigskip
\bigskip

\begin{center}
\begin{tabular}{ clc } 
% \hline
 \hspace*{0.3in}{\bf Appendix\hspace*{0.3in}} & \hspace*{0.3in}{\bf Title}& {\bf Page Number}  \\ 
% \hline
\\
 A &  Making Fewer Proposals: Proof of Theorem \ref{lem::acceptable-suffice} &  \pageref{sec::fewer-props}\\ \\
% \hline
% B &  Technical Lemmas& \pageref{sec::technical}\\ 
% \hline
 B &  Proof of the Key Lemma (Lemma~\ref{lem::key_bounded})& \pageref{sec::main_lemma_full_proof}\\
% \hline
\\
 C &  Proofs of the Upper Bounds in Section \ref{sec::results}& \pageref{sec::upper_full_proofs}\\
% \hline
\\ D & Range of Public Ratings for Acceptable Edges &
\pageref{sec::cone-size}\\
% \hline
\\
 E &  Proofs of Lower Bounds in Section \ref{sec::results}& \pageref{sec::lower_full_proofs}\\
% \hline
\\
 F &  Distribution Bound on Losses: Proof of Theorem~\ref{thm::distr-bound} & \pageref{sec::dist-bound}\\
% \hline
\\
 G &  $\epsilon$-Bayes-Nash Equilibria & \pageref{sec::eps-BN-equil-full-match}\\
% \hline
\\
 H &  Additional Numerical Experiments& \pageref{sec::more_numerics}\\
% \hline
\end{tabular}
\end{center}
